# Supplementary material for: Printable Aggregate Elements
Source: arXiv:1811.02626 source file (2018-11-06)
Supplement: Supplementary file 1 [file 01-derivatives.tex]

%%%%%%%%%%%%%%%%%%%%%%%%%%%%%%%%%%%%%%%%%%%%%%%%%%%%%%%%%%%%%%%%%%%%%%%%%%%%%%%%
\section{Sensitivity Analysis}

In this section we describe in more details how to compute the partial derivatives in order to perform gradient-descent optimization on our objective function.
Recall our general computation pipeline
\begin{align}
	\allDofs
	\stackrel{\dofsToSamplePos}{\to} \allSamplePos
	\stackrel{\samplePosToDensities}{\to} \allDensities
	\stackrel{\densitiesToScalar}{\to} \compliance
\end{align}

And the chain-rule for computing the gradient of our objective function $\densitiesToScalar \circ \samplePosToDensities \circ \dofsToSamplePos \colon \allDofs \to \compliance(\allDofs)$
\begin{align}
	\grad{(\densitiesToScalar \circ \samplePosToDensities \circ \dofsToSamplePos)} =
		\grad{\densitiesToScalar} \;
		\jacobianMatrix{\samplePosToDensities} \;
		\jacobianMatrix{\dofsToSamplePos}
	\label{eq:chain-rule-jacobian}
\end{align}

In \Cref{subsec:material-densities}, we explain how to compute the material density derivative necessary to compute $\jacobianMatrix{\samplePosToDensities}$.
In \Cref{subsuc:sample-positions}, we detail to compute $\jacobianMatrix{\dofsToSamplePos}$ for elements parameterized by a rigid transformation (translation + rotation).
Finally, in \Cref{subsec:deformable-elements}, we extent the discussion about $\jacobianMatrix{\dofsToSamplePos}$ to elements that can deform during the optimization.

Note that in general, the Jacobian matrices $\jacobianMatrix{\samplePosToDensities}$ and $\jacobianMatrix{\dofsToSamplePos}$ are sparse or upper-triangular, so the product in \Cref{eq:chain-rule-jacobian} can be computed efficiently.

%%%%%%%%%%%%%%%%%%%%%%%%%%%%%%%%%%%%%%%%
\subsection{Material Densities}
\label{subsec:material-densities}

Recall the definition of smoothed step function that we use in our algorithm:
\begin{align}
	\densitySampleFunc(\currentPosition) =
	\frac{1}{2} + \frac{1}{2} \tanh( \rbfSlope \left(
		\sampleRadius^2
		- \left(\frac{\norm{\currentPosition - \samplePosition}}{\rbfWidth}\right)^2
	\right) )
	\label{eq:material-densities:heaviside}
\end{align}

Let $u = \norm{\currentPosition - \samplePosition}^2$. We can rewrite $\densitySampleFunc(\currentPosition)$ as a function of $u$, which gives the following formula:

\begin{align}
	\grad{\densitySampleFunc(\currentPosition)} = 2 \currentPosition \pderivative{\densitySampleFunc}{r}
\end{align}
where
\begin{align}
	\pderivative{\densitySampleFunc}{u} =
		- \beta \frac{1}{2 \alpha^2} \left(
			1-\tanh(\beta \left(\sampleRadius^2 - \frac{u}{\alpha^2}\right))^2
		\right)
\end{align}
% From my code:
% f = 0.5 + 0.5 * tanh(beta * (r2 - x2 / alpha^2))
% f' = df/dx2 = -0.5*beta*(-tanh(beta*(r2 - x2/alpha**2))**2 + 1)/alpha**2

%%%%%%%%%%%%%%%%%%%%%%%%%%%%%%%%%%%%%%%%
\subsection{Sample Positions}
\label{subsuc:sample-positions}

For a given element $\element$ and a sample $\sample \in \allSamplesElement$, we seek to compute the sensitivities of the sample position $\samplePosition$ with respect to the element parameters $\allDofsElement$. Recall that the sample positions are computed via the following equation

\begin{align}
	\allSamplePosElement(\allDofsElement) = \elementRotation(\allDofsElement) \elementLinear \allDofsSamplePos(\allDofsElement) + \elementTranslation(\allDofsElement)
\end{align}

Or, if we let $\dofsSamplePos_\sample = \allDofsSamplePos[:\,, \sample] \in \reals^{\dimension \times 1}$ be the untransformed position of the sample $\sample$:

\begin{align}
	\samplePosition(\allDofsElement) = \elementRotation(\allDofsElement) \elementLinear \dofsSamplePos_\sample(\allDofsElement) + \elementTranslation(\allDofsElement)
\end{align}

In the most general case, the parameters of an element $\element$ can be expressed as
\begin{align}
	\allDofsElement
		&= (\theta_1, \ldots, \theta_{\size{\allDofsElement}})\\
		&= (\dofTranslation_1, \ldots, \dofTranslation_\dimension, \dofRotation_1, \ldots, \dofRotation_{\size{\dofsRotation}}, \dofSamplePos_{11}, \ldots, \dofSamplePos_{\size{\dofsSamplePos}\dimension})
\end{align}
where $\dofsTranslation = (\dofTranslation_1, \ldots, \dofTranslation_\dimension)$ stands for the translation of the element centroid in dimension $\dimension$,
$\dofsRotation = (\dofRotation_1, \ldots, \dofRotation_{\size{\dofsRotation}})$ are the parameters of the rotation ($\size{\dofsRotation} = 1$ in 2D, $\size{\dofsRotation} = 3$ in 3D),
and $\dofsSamplePos = (\dofSamplePos_{11}, \ldots, \dofSamplePos_{\size{\dofsSamplePos}\dimension}))$ are the sample coordinates in the untransformed configuration.
Finally, $\elementLinear$ encodes a fixed linear transformation (rotation + scaling) that is fixed for a given element.

To compute the partial derivative
\begin{align}
	\pderivative{\samplePosition}{\oneDof{k}} \in \reals^{\dimension \times 1}
	\label{eq:sample-position-pderiv-general}
\end{align}

We distinguish between the following cases for $\theta_k$:

%---------------------------------------
\paragraph{Translation}
When $\theta_k = \dofTranslation_i$, we get
\begin{align}
	\pderivative{\samplePosition}{\dofTranslation_i}
		= [\delta_{ij}]_j
\end{align}
where $\delta_{ij}$ is the Kronecker delta symbol.

%---------------------------------------
\paragraph{Rotation}
When $\theta_k = \dofRotation_i$, we get
\begin{align}
	\pderivative{\samplePosition}{\dofRotation_i}
		= \pderivative{\elementRotation}{\dofRotation_i}
		\elementLinear \dofsSamplePos_\sample
\end{align}
since $\dofsSamplePos_\sample$ is constant with respect to $\dofRotation_i$.
In 3D, the partial derivative of the rotation matrix $\pderivative{\elementRotation}{\dofRotation_i}$ with respect to the exponential map parameters can be computed following \cite{Grassia:1998:PPO,Gallego:2015:ACF}.

%---------------------------------------
\paragraph{Sample Positions}
When $\theta_k = \dofSamplePos_{\otherSample i}$, we get
\begin{align}
	\pderivative{\samplePosition}{\dofSamplePos_{\otherSample i}} =
	\begin{cases}
		\elementRotation(\allDofsElement) \elementLinear [\delta_{ij}]_j
		& \text{if } \sample = \otherSample \\
		0
		& \text{if } \sample \neq \otherSample
	\end{cases}
	\label{eq:sample-position-pderiv-sample}
\end{align}

Note that in practice, we do not use the sample positions $\allDofsSamplePos$ directly as degrees of freedom, but we parameterize them as explained in \Cref{subsec:deformable-elements} for elements that are allowed to deform.

%%%%%%%%%%%%%%%%%%%%%%%%%%%%%%%%%%%%%%%%
\subsection{Deformable Elements}
\label{subsec:deformable-elements}

For elements that are allowed to deform during the optimization process, recall that the sample positions in the local reference frame are defined as (see \Cref{fig:deformable-parameterization}):
\begin{align}
	\dofsSamplePos_\sample \eqdef \rotationMatrix(\dofsAngularPos_\sample) \deltaSamplePos_\sample + \dofsSamplePos_{\parent{\sample}}
	\label{eq:dof-sample-pos-param}
\end{align}
where $\parent{\sample}$ is the parent node of sample $\sample$ in a rooted tree $\rootedTreeElement$ connecting the samples within an element $\element$. In this case, we seek to evaluate $\pderivative{\samplePosition}{\theta_k}$ (\Cref{eq:sample-position-pderiv-general}) in the case where $\oneDof{k} = \dofAngularPos_{\otherSample_i}$, and where $\dofsAngularPos_\otherSample = (\dofAngularPos_{\otherSample_1}, \dofAngularPos_{\otherSample_2}, \dofAngularPos_{\otherSample_3})$ are the exponential map coefficients for the rotation describing $\dofsSamplePos_\otherSample$ in \Cref{eq:dof-sample-pos-param}.

\input{figs/deformable-parameterization}

We can write
\begin{align}
	\pderivative{\samplePosition}{\dofSamplePos_{\otherSample i}}
		= \elementRotation(\allDofsElement) \elementLinear
		\pderivative{\dofsSamplePos_{\sample}}{\dofAngularPos_{\otherSample i}}
\end{align}

And from \Cref{eq:dof-sample-pos-param} we can write that
\begin{align}
	\pderivative{\dofsSamplePos_{\sample}}{\dofAngularPos_{\otherSample i}}
		= \pderivative{\rotationMatrix(\dofsAngularPos_\sample)}{\dofAngularPos_{\otherSample i}}
		\deltaSamplePos_\sample
		+ \pderivative{\dofsSamplePos_{\parent{\sample}}}{\dofAngularPos_{\otherSample i}}
	\label{eq:dof-sample-pos-pderiv}
\end{align}

From \Cref{eq:dof-sample-pos-pderiv} it can be seen that $\pderivative{\dofsSamplePos_{\sample}}{\dofAngularPos_{\otherSample i}}$ is non-zero iff $\sample$ is a descendant of $\otherSample$ in the rooted tree $\rootedTreeElement$, in which case we write $\sample \in \successors{\otherSample}$.

Note that \Cref{eq:dof-sample-pos-pderiv} also implies that the Jacobian $\jacobianMatrix{\dofsToSamplePos}$ is not sparse anymore, but we can still reindex the samples in order to make it upper-triangular per element.

Let $\samplePosToScalar = \densitiesToScalar \circ \samplePosToDensities$.
In order to compute the vector-matrix product $\grad{\samplePosToScalar} \; \jacobianMatrix{\dofsToSamplePos}$ efficiently (i.e. linearly in $\size{\grad{\samplePosToScalar}}$), one can propagate partial sums in backward topological order of $\rootedTreeElement$, i.e. starting from the leaves and going up to the root.

More precisely, when $\oneDof{k} = \dofAngularPos_{\otherSample i}$ we have
\begin{align}
	\grad{(\samplePosToScalar \circ \dofsToSamplePos)}_k
		& = \sum_{\sample \in \allSamples}
			\grad{(\samplePosToScalar)}_\sample
			\pderivative{\samplePosition}{\oneDof{k}}\\
		& =
			\elementRotation(\allDofsElement) \elementLinear
			\sum_{\sample \in \allSamples}
			\grad{(\samplePosToScalar)}_\sample
			\pderivative{\dofsSamplePos_{\sample}}{\dofAngularPos_{\otherSample i}}
\end{align}

From the recursive formulation in \eqref{eq:dof-sample-pos-pderiv}, we deduce that
\begin{align}
	\sum_{\sample \in \allSamples}
		\grad{(\samplePosToScalar)}_\sample
		\pderivative{\dofsSamplePos_{\sample}}{\dofAngularPos_{\otherSample i}}
	= \left(
		\sum_{\sample \in \successors{\otherSample}}
		\grad{(\samplePosToScalar)}_\sample)
	\right)
	\pderivative{\rotationMatrix(\dofsAngularPos_\otherSample)}{\dofAngularPos_{\otherSample i}}
		\deltaSamplePos_\otherSample
\end{align}

Finally, the partial sum $\sum_{\sample \in \successors{\otherSample}} \grad{(\samplePosToScalar)}_\sample)$ can be computed efficiently with dynamic programming by performing a traversal of the samples in $\rootedTreeElement$ in backward topological order (i.e. starting from the leaves).

%%%%%%%%%%%%%%%%%%%%
\subsubsection{Computing \texorpdfstring{$\rootedTreeElement$}{T^e}}
\label{subsubsec:tree-computation}

Since our algorithm takes as input a surface or volumetric mesh, and sample control points inside their volume, we need to be able to define tree $\rootedTreeElement$ connecting the samples together.
We use a very simple heuristic that works well in practice, and simply define $\rootedTreeElement$ as the minimum covering tree of a Delaunay triangulation of the sample positions $\allDofsSamplePos$, where each edge is weighted by the distance between the two samples.

In order to find a suitable root for $\rootedTreeElement$, representing the anchor point from which the other sample positions are derived, we simply choose the vertex $y_0$ that minimize the maximum height of the resulting rooted tree.
While the graph $\rootedTreeElement$ for an element is typically small ($\leq 100$ samples in our experiments), and the value of $y_0$ could be brute-forced, an efficient way to find $y_0$ is to take the vertex at half the diameter of $\rootedTreeElement$ as follows:
\begin{enumerate}
	\item Start from any vertex $x \in \rootedTreeElement$.
	\item Compute $y \gets \textsc{Furthest}[x]$, most distant vertex from $x$, with a DFS.
	\item Compute again $z \gets \textsc{Furthest}[y]$.
	\item Backtrack by half the diameter from $z$, set this vertex as the root $y_0$.
\end{enumerate}
