# Supplementary material for: Printable Aggregate Elements
Source: arXiv:1811.02626 ancillary file (2018-11-06)
Supplement: Supplementary file 2 [file supplemental.pdf]

# Printable Aggregate Elements

## Supplemental Material

JÉRÉMIE DUMAS, INRIA, University of Hong Kong, nTopology

SYLVAIN LEFEBVRE, INRIA, Université de Lorraine

LI-YI WEI, University of Hong Kong

### 1 NOTATION SUMMARY

We summarize below the notations used throughout our paper:

|                           |                                                               |
|---------------------------|---------------------------------------------------------------|
| $\Theta$                  | Element parameters (degrees of freedom).                      |
| $\mathbf{t}$              | Translation parameters for an element.                        |
| $\gamma$                  | Rotation parameters (exp. map coefficients) for an element.   |
| $\mathbf{y}$              | Untransformed sample positions (local element coordinates).   |
| $\omega_s$                | Exp. map coefficients for a sample $s$ in a flexible element. |
| $\mathbf{P}$              | World-space sample positions (in matrix form).                |
| $\rho_s$                  | Continuous material density RBF (per sample).                 |
| $\rho$                    | Continuous material density ( $\max_s \rho_s$ ).              |
| $\mathbf{G}$              | Discretized grid where the elements are embedded.             |
| $\mathbf{x}$              | Grid cell densities (integrated from $\rho$ ).                |
| $\mathbf{u}$              | Grid displacements (nodal values).                            |
| $\mathbf{f}_{\text{ext}}$ | User-defined external forces (nodal values).                  |
| $C$                       | Compliance function (scalar value).                           |

Table 1. List of symbols.

### 2 SENSITIVITY ANALYSIS

In this section we describe in more details how to compute the partial derivatives in order to perform gradient-descent optimization on our objective function. Recall our general computation pipeline

$$\Theta \xrightarrow{h} \mathbf{P} \xrightarrow{g} \mathbf{x} \xrightarrow{f} C \quad (1)$$

And the chain-rule for computing the gradient of our objective function  $f \circ g \circ h: \Theta \rightarrow C(\Theta)$

$$\nabla(f \circ g \circ h) = \nabla f \mathbf{J}_g \mathbf{J}_h \quad (2)$$

In Section 2.1, we explain how to compute the material density derivative necessary to compute  $\mathbf{J}_g$ . In Section 2.2, we detail to compute  $\mathbf{J}_h$  for elements parameterized by a rigid transformation (translation + rotation). Finally, in Section 2.3, we extend the discussion about  $\mathbf{J}_h$  to elements that can deform during the optimization.

Note that in general, the Jacobian matrices  $\mathbf{J}_g$  and  $\mathbf{J}_h$  are sparse or upper-triangular, so the product in Equation (2) can be computed efficiently.

#### 2.1 Material Densities

Recall the definition of smoothed step function that we use in our algorithm:

$$\rho_s(\mathbf{p}) = \frac{1}{2} + \frac{1}{2} \tanh\left(\beta\left(r_s^2 - \left(\frac{\|\mathbf{p} - \mathbf{p}_s\|}{\alpha}\right)^2\right)\right) \quad (3)$$

Let  $u = \|\mathbf{p} - \mathbf{p}_s\|^2$ . We can rewrite  $\rho_s(\mathbf{p})$  as a function of  $u$ , which gives the following formula:

$$\nabla \rho_s(\mathbf{p}) = 2\mathbf{p} \frac{\partial \rho_s}{\partial r} \quad (4)$$

where

$$\frac{\partial \rho_s}{\partial u} = -\beta \frac{1}{2\alpha^2} \left(1 - \tanh\left(\beta\left(r_s^2 - \frac{u}{\alpha^2}\right)\right)\right)^2 \quad (5)$$

#### 2.2 Sample Positions

For a given element  $e$  and a sample  $s \in \mathcal{S}^e$ , we seek to compute the sensitivities of the sample position  $\mathbf{p}_s$  with respect to the element parameters  $\Theta^e$ . Recall that the sample positions are computed via the following equation

$$\mathbf{P}^e(\Theta^e) = \mathbf{R}^e(\Theta^e) \mathbf{A}^e \mathbf{Y}(\Theta^e) + \mathbf{T}^e(\Theta^e) \quad (6)$$

Or, if we let  $\mathbf{y}_s = \mathbf{Y}[:, s] \in \mathbb{R}^{d \times 1}$  be the untransformed position of the sample  $s$ :

$$\mathbf{p}_s(\Theta^e) = \mathbf{R}^e(\Theta^e) \mathbf{A}^e \mathbf{y}_s(\Theta^e) + \mathbf{T}^e(\Theta^e) \quad (7)$$

In the most general case, the parameters of an element  $e$  can be expressed as

$$\Theta^e = (\theta_1, \dots, \theta_{|\Theta^e|}) \quad (8)$$

$$= (t_1, \dots, t_d, \gamma_1, \dots, \gamma_{|\gamma|}, y_{11}, \dots, y_{|\gamma|d}) \quad (9)$$

where  $\mathbf{t} = (t_1, \dots, t_d)$  stands for the translation of the element centroid in dimension  $d$ ,  $\gamma = (\gamma_1, \dots, \gamma_{|\gamma|})$  are the parameters of the rotation ( $|\gamma| = 1$  in 2D,  $|\gamma| = 3$  in 3D), and  $\mathbf{y} = (y_{11}, \dots, y_{|\gamma|d})$  are the sample coordinates in the untransformed configuration. Finally,  $\mathbf{A}^e$  encodes a fixed linear transformation (rotation + scaling) that is fixed for a given element.

To compute the partial derivative

$$\frac{\partial \mathbf{p}_s}{\partial \theta_k} \in \mathbb{R}^{d \times 1} \quad (10)$$

We distinguish between the following cases for  $\theta_k$ :

**Translation.** When  $\theta_k = t_i$ , we get

$$\frac{\partial \mathbf{p}_s}{\partial t_i} = [\delta_{ij}]_j \quad (11)$$

where  $\delta_{ij}$  is the Kronecker delta symbol.

**Rotation.** When  $\theta_k = \gamma_i$ , we get

$$\frac{\partial \mathbf{p}_s}{\partial \gamma_i} = \frac{\partial \mathbf{R}^e}{\partial \gamma_i} \mathbf{A}^e \mathbf{y}_s \quad (12)$$

since  $\mathbf{y}_s$  is constant with respect to  $\gamma_i$ . In 3D, the partial derivative of the rotation matrix  $\frac{\partial \mathbf{R}^e}{\partial \gamma_i}$  with respect to the exponential map parameters can be computed following [Grassia 1998; Gallego and Yezzi 2015].

**Sample Positions.** When  $\theta_k = y_{s'i}$ , we get

$$\frac{\partial \mathbf{p}_s}{\partial y_{s'i}} = \begin{cases} \mathbf{R}^e(\Theta^e) \mathbf{A}^e [\delta_{ij}]_j & \text{if } s = s' \\ 0 & \text{if } s \neq s' \end{cases} \quad (13)$$

Note that in practice, we do not use the sample positions  $\mathbf{Y}$  directly as degrees of freedom, but we parameterize them as explained in Section 2.3 for elements that are allowed to deform.

### 2.3 Deformable Elements

For elements that are allowed to deform during the optimization process, recall that the sample positions in the local reference frame are defined as (see Figure 1):

$$\mathbf{y}_s \stackrel{\text{def}}{=} \mathbf{R}(\omega_s) \delta_s + \mathbf{y}_{\text{pred}[s]} \quad (14)$$

where  $\text{pred}[s]$  is the parent node of sample  $s$  in a rooted tree  $\mathcal{T}^e$  connecting the samples within an element  $e$ . In this case, we seek to evaluate  $\frac{\partial \mathbf{p}_s}{\partial \theta_k}$  (Equation (10)) in the case where  $\theta_k = \omega_{s'i}$ , and where  $\omega_{s'} = (\omega_{s'_1}, \omega_{s'_2}, \omega_{s'_3})$  are the exponential map coefficients for the rotation describing  $\mathbf{y}_{s'}$  in Equation (14).

We can write

$$\frac{\partial \mathbf{p}_s}{\partial y_{s'i}} = \mathbf{R}^e(\Theta^e) \mathbf{A}^e \frac{\partial \mathbf{y}_s}{\partial \omega_{s'i}} \quad (15)$$

And from Equation (14) we can write that

$$\frac{\partial \mathbf{y}_s}{\partial \omega_{s'i}} = \frac{\partial \mathbf{R}(\omega_s)}{\partial \omega_{s'i}} \delta_s + \frac{\partial \mathbf{y}_{\text{pred}[s]}}{\partial \omega_{s'i}} \quad (16)$$

From Equation (16) it can be seen that  $\frac{\partial \mathbf{y}_s}{\partial \omega_{s'i}}$  is non-zero iff  $s$  is a descendant of  $s'$  in the rooted tree  $\mathcal{T}^e$ , in which case we write  $s \in \text{succ}[s']$ .

Note that Equation (16) also implies that the Jacobian  $\mathbf{J}_h$  is not sparse anymore, but we can still reindex the samples in order to make it upper-triangular per element.

Let  $fg = f \circ g$ . In order to compute the vector-matrix product  $\nabla fg \mathbf{J}_h$  efficiently (i.e. linearly in  $|\nabla fg|$ ), one can propagate partial

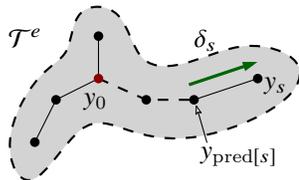

Fig. 1. *Deformable element parameterization.* The position of a sample dof is expressed hierarchically as in ???. The root sample position is fixed in the local coordinate system of the element.

sums in backward topological order of  $\mathcal{T}^e$ , i.e. starting from the leaves and going up to the root.

More precisely, when  $\theta_k = \omega_{s'i}$  we have

$$\nabla(fg \circ h)_k = \sum_{s \in \mathcal{S}} \nabla(fg)_s \frac{\partial \mathbf{p}_s}{\partial \theta_k} \quad (17)$$

$$= \mathbf{R}^e(\Theta^e) \mathbf{A}^e \sum_{s \in \mathcal{S}} \nabla(fg)_s \frac{\partial \mathbf{y}_s}{\partial \omega_{s'i}} \quad (18)$$

From the recursive formulation in (16), we deduce that

$$\sum_{s \in \mathcal{S}} \nabla(fg)_s \frac{\partial \mathbf{y}_s}{\partial \omega_{s'i}} = \left( \sum_{s \in \text{succ}[s']} \nabla(fg)_s \right) \frac{\partial \mathbf{R}(\omega_{s'})}{\partial \omega_{s'i}} \delta_{s'} \quad (19)$$

Finally, the partial sum  $\sum_{s \in \text{succ}[s']} \nabla(fg)_s$  can be computed efficiently with dynamic programming by performing a traversal of the samples in  $\mathcal{T}^e$  in backward topological order (i.e. starting from the leaves).

**2.3.1 Computing  $\mathcal{T}^e$ .** Since our algorithm takes as input a surface or volumetric mesh, and sample control points inside their volume, we need to be able to define tree  $\mathcal{T}^e$  connecting the samples together. We use a very simple heuristic that works well in practice, and simply define  $\mathcal{T}^e$  as the minimum covering tree of a Delaunay triangulation of the sample positions  $\mathbf{Y}$ , where each edge is weighted by the distance between the two samples.

In order to find a suitable root for  $\mathcal{T}^e$ , representing the anchor point from which the other sample positions are derived, we simply choose the vertex  $y_0$  that minimize the maximum height of the resulting rooted tree. While the graph  $\mathcal{T}^e$  for an element is typically small ( $\leq 100$  samples in our experiments), and the value of  $y_0$  could be brute-forced, an efficient way to find  $y_0$  is to take the vertex at half the diameter of  $\mathcal{T}^e$  as follows:

- (1) Start from any vertex  $x \in \mathcal{T}^e$ .
- (2) Compute  $y \leftarrow \text{FURTHEST}[x]$ , most distant vertex from  $x$ , with a DFS.
- (3) Compute again  $z \leftarrow \text{FURTHEST}[y]$ .
- (4) Backtrack by half the diameter from  $z$ , set this vertex as the root  $y_0$ .

### REFERENCES

- G. Gallego and A. Yezzi. 2015. A Compact Formula for the Derivative of a 3-D Rotation in Exponential Coordinates. *Journal of Mathematical Imaging and Vision* 51, 3 (03 2015), 378–384. <https://doi.org/10.1007/s10851-014-0528-x>
- F. S. Grassia. 1998. Practical Parameterization of Rotations Using the Exponential Map. *Journal of Graphics Tools* 3, 3 (01 1998), 29–48. <https://doi.org/10.1080/10867651.1998.10487493>
