# Supplementary material for: Printable Aggregate Elements
Source: arXiv:1811.02626 source file (2018-11-06)
Supplement: Supplementary file 3 [file 02-notations.tex]

%%%%%%%%%%%%%%%%%%%%%%%%%%%%%%%%%%%%%%%%%%%%%%%%%%%%%%%%%%%%%%%%%%%%%%%%%%%%%%%%
\section{Notation Summary}

We summarize below the notations used throughout our paper:

\begin{table}[htbp]
	\begin{tabular}{cl}
		$\allDofs$ & Element parameters (degrees of freedom). \\
		$\dofsTranslation$ & Translation parameters for an element. \\
		$\dofsRotation$ & Rotation parameters (exp. map coefficients) for an element. \\
		$\dofsSamplePos$ & Untransformed sample positions (local element coordinates). \\
		$\dofsAngularPos_\sample$ & Exp. map coefficients for a sample $\sample$ in a flexible element. \\
		$\allSamplePos$ & World-space sample positions (in matrix form). \\
		$\densitySampleFunc$ & Continuous material density RBF (per sample). \\
		$\densityAllSamples$ & Continuous material density ($\max_\sample \densitySampleFunc$). \\
		$\allGridCells$ & Discretized grid where the elements are embedded. \\
		$\allDensities$ & Grid cell densities (integrated from $\densityAllSamples$). \\
		$\displacements$ & Grid displacements (nodal values). \\
		$\externalForces$ & User-defined external forces (nodal values). \\
		$\compliance$ & Compliance function (scalar value).
	\end{tabular}

	\caption{
		List of symbols.
	}
	\label{tab:timings}
\end{table}
